# Supplementary material for: Surface Networks
Source: arXiv:1705.10819 source file (2018-06-18)
Supplement: Supplementary file 1 [file nips_supplementary.tex]

\documentclass{article}

% if you need to pass options to natbib, use, e.g.:
% \PassOptionsToPackage{numbers, compress}{natbib}
% before loading nips_2017
%
% to avoid loading the natbib package, add option nonatbib:
% \usepackage[nonatbib]{nips_2017}

\usepackage{nips_2017}

% to compile a camera-ready version, add the [final] option, e.g.:
% \usepackage[final]{nips_2017}

\usepackage[utf8]{inputenc} % allow utf-8 input
\usepackage[T1]{fontenc}    % use 8-bit T1 fonts
\usepackage{hyperref}       % hyperlinks
\usepackage{url}            % simple URL typesetting
\usepackage{booktabs}       % professional-quality tables
\usepackage{amsfonts}       % blackboard math symbols
\usepackage{nicefrac}       % compact symbols for 1/2, etc.
\usepackage{microtype}      % microtypography
\usepackage{amsmath,graphicx}
\usepackage{amssymb}
\usepackage{amsthm}
\usepackage{enumitem}
\usepackage{overpic}
\usepackage{color}
\usepackage{tikz}

\title{Supplementary Material for Paper Surface Networks}

% The \author macro works with any number of authors. There are two
% commands used to separate the names and addresses of multiple
% authors: \And and \AND.
%
% Using \And between authors leaves it to LaTeX to determine where to
% break the lines. Using \AND forces a line break at that point. So,
% if LaTeX puts 3 of 4 authors names on the first line, and the last
% on the second line, try using \AND instead of \And before the third
% author name.

\author{
  Ilya Kostrikov \\
  Courant Institute of Mathematical Sciences\\
  New York University\\
  New York, NY, 10011 \\
 \And
    Joan Bruna \\
  Courant Institute of Mathematical Sciences\\
  New York University\\
  New York, NY, 10011 \\
 \And
    Daniele Panozzo \\
  Courant Institute of Mathematical Sciences\\
  New York University\\
  New York, NY, 10011 
\And
    Denis Zorin \\
  Courant Institute of Mathematical Sciences\\
  New York University\\
  New York, NY, 10011 
}
  %% examples of more authors
  %% \And
  %% Coauthor \\
  %% Affiliation \\
  %% Address \\
  %% \texttt{email} \\
  %% \AND
  %% Coauthor \\
  %% Affiliation \\
  %% Address \\
  %% \texttt{email} \\
  %% \And
  %% Coauthor \\
  %% Affiliation \\
  %% Address \\
  %% \texttt{email} \\
  %% \And
  %% Coauthor \\
  %% Affiliation \\
  %% Address \\
  %% \texttt{email} \\

\begin{document}
% \nipsfinalcopy is no longer used

\maketitle

\begin{abstract}

\end{abstract}

\input{dirac}

\input{proof}

\input{furtherexps}

\newpage

\bibliography{biblio}
\bibliographystyle{plain}

\end{document}
